# Supplementary material for: 3D Single-port Labyrinthine Acoustic Metamaterial
Source: arXiv:1608.04599 source file (2016-08-11)
Supplement: Supplementary file 1 [file SupplementaryHu.pdf]

# 3D Single-port Labyrinthine Acoustic Metamaterial (Supplementary Information)

Chi Zhang[1] and Xinhua Hu[1]

[1]*Department of Materials Science, Key Laboratory of Micro- and Nano-Photonic Structures (Ministry of Education), and Laboratory of Advanced Materials, Fudan University, Shanghai 200433, China*

## I. Coupled mode theory

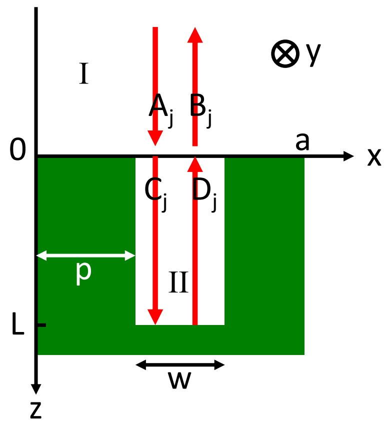


Consider the 2D acoustic metasurface shown in the right pannel of Fig. 1a, which is invariant in the $y$ direction and periodic along the $x$ direction (only a unit cell of the metasurface is replotted above). The green part is rigid body. Fluid 1 exists in region I with $z < 0$ and $0 < x < a$ (*i.e.* background), while fluid 2 exists in region II with $z < 0$ and $p < x < p + w$ (*i.e.* channel).

In region I, the acoustic pressure $P_1(z, x)$ satisfies $\nabla^2 P_1 + k_1^2 P_1 = 0$, so that we have

$$P_1 = \sum_{j=-N_1}^{N_1} [C_j \exp(ik_{1zj}z) + D_j \exp(-ik_{1zj}z)] \exp(ik_{1xj}x) \text{ for } z < 0 \text{ and } 0 < x < a, \quad \text{(S1)}$$

where $k_1 = \omega/c_1$, $c_1 = \sqrt{B_1/\rho_1}$, $B_1$, and $\rho_1$ are the wavenumber, sound velocity, bulk modulus, and mass density in region I, respectively, $k_{1z}^2 + k_{1x}^2 = k_1^2$, and $k_{1x} = j2\pi/a$ with $j = 0, \pm1, \pm2, \cdots, \pm N_1$.

In region II, the acoustic pressure $P_1(z, x)$ satisfies $\nabla^2 P_2 + k_2^2 P_2 = 0$ with $\partial_x P_2 = 0$ at $x = p$ and $p + w$. Hence, we have

$$P_2 = \sum_{j=0}^{N_2} [E_j \exp(ik_{2zj}z) + F_j \exp(-ik_{2zj}z)] \cos[k_{2xj}(x - p)] \text{ for } z > 0 \text{ and } p < x < p + w, \quad \text{(S2)}$$

where $k_2 = \omega/c_2$, $c_2 = \sqrt{B_2/\rho_2}$, $B_2$, and $\rho_2$ are the wavenumber, sound velocity, bulk modulus, and mass density in region I, respectively, $k_{2z}^2 + k_{2x}^2 = k_2^2$, and $k_{1x} = j\pi/a$ with $j = 0, 1, 2, \cdots, N_2$.

The linking conditions at $z = 0$ are

$$P_1 = P_2 \text{ for } p < x < p + w, \quad \text{(S3)}$$

$$\rho_1^{-1}\frac{\partial}{\partial z}P_1 = \left\{ \begin{array}{c} 0 \text{ for } p > x \text{ or } x > p+w \\ \rho_2^{-1}\frac{\partial}{\partial z}P_2 \text{ for } p < x < p+w \end{array} \right\}. \tag{S4}$$

By substituting Eqs. (S1) and (S2) into Eqs. (S3) and (S4), and then multiplying Eq. (S3) with $\int_p^{p+w}\cos\left[k_{2xl}\left(x-p\right)\right]dx$ ($l_2 = 0, 1, 2, \cdots, N_2$) and Eq. (S4) with $\int_0^a \exp\left(-ik_{1xl}x\right)dx$ ($l_1 = 0, \pm1, \pm2, \cdots, \pm N_1$), we have

$$\sum_{j=-N_1}^{N_1} G_{1,l_2j}\left(C_j + D_j\right) = \sum_{j=0}^{N_2} G_{2,l_2j}\left(E_j + F_j\right) \text{ with } l_2 = 0, 1, 2, \cdots, N_2, \tag{S5}$$

$$\sum_{j=-N_1}^{N_1} G_{3,l_1j}\left(C_j - D_j\right) = \sum_{j=0}^{N_2} G_{4,l_1j}\left(E_j - F_j\right) \text{ with } l_1 = 0, \pm1, \pm2, \cdots, \pm N_1, \tag{S6}$$

where $G_{1,l_2j} = \int_p^{p+w}\cos\left[k_{2xl_2}\left(x-p\right)\right]\exp\left(ik_{1xj}x\right)dx$, $G_{2,l_2j} = \int_p^{p+w}\cos\left[k_{2xl_2}\left(x-p\right)\right]\cos\left[k_{2xj}\left(x-p\right)\right]dx$, $G_{3,l_1j} = k_{1zj}\rho_1^{-1}\int_0^a \exp\left(-ik_{1xl_1}x\right)\exp\left(ik_{1xj}x\right)dx$, and $G_{4,l_1j} = \rho_2^{-1}k_{2zj}\int_p^{p+w}\exp\left(-ik_{1xl_1}x\right)\cos\left[k_{2xj}\left(x-p\right)\right]dx$. Since $F_j = E_j\exp\left(i2k_{2zj}L\right)$, we have

$$\sum_{j=-N_1}^{N_1} G_{1,l_2j}\left(C_j + D_j\right) = \sum_{j=0}^{N_2} G_{2,l_2j}\left[1 + \exp\left(i2k_{2zj}L\right)\right]E_j \text{ with } l_2 = 0, 1, 2, \cdots, N_2, \tag{S7}$$

$$\sum_{j=-N_1}^{N_1} G_{3,l_1j}\left(C_j - D_j\right) = \sum_{j=0}^{N_2} G_{4,l_1j}\left[1 - \exp\left(i2k_{2zj}L\right)\right]E_j \text{ with } l_1 = 0, \pm1, \pm2, \cdots, \pm N_1. \tag{S8}$$

By using $C_j = \delta_{j,0}$, $D_j$, $E_j$, reflection $R = \left|D_0/C_0\right|^2$, and absorption $A = 1 - R$ can be obtained.

## II. Derivation of Eq. (1)

When $N_1 = N_2 = 0$, Eqs. (S7) and (S8) become as

$$G_1\left(C + D\right) = G_2\left[1 + \exp\left(i2k_2L\right)\right]E, \tag{S9}$$

$$G_3\left(C - D\right) = G_4\left[1 - \exp\left(i2k_2L\right)\right]E, \tag{S10}$$

where $G_1 = h$, $G_2 = h$, $G_3 = k_1\rho_1^{-1}a$, $G_4 = k_2\rho_2^{-1}w$. Hence, we have

$$R \equiv \left|\frac{D}{C}\right|^2 = \left|\frac{1-Z}{1+Z}\right|^2, \tag{S11}$$

$$Z = \frac{k_2\rho_2^{-1}w\left[1 - \exp\left(i2k_2L\right)\right]}{k_1\rho_1^{-1}a\left[1 + \exp\left(i2k_2L\right)\right]} \overset{k_2\rho_2^{-1}\simeq k_1\rho_1^{-1}}{=} \frac{w\left[1 - \exp\left(i2k_2L\right)\right]}{a\left[1 + \exp\left(i2k_2L\right)\right]}. \tag{S12}$$

We note that Eq. (1) can be obtained from Eqs. (S11) and (S12).

## III. Derivation of Eqs. (2) and (3)

The condition for $R = 0$ (or $Z = 1$) is

$$\exp(i2k_2L) = -(1 - w/a)/(1 + w/a) \tag{S13}$$

By using $k_2 = k_1(1 + i\beta)$ and thus $\exp(i2k_2L) = \exp(i2k_1L)\exp(-2k_1\beta L)$, the above equation becomes as $\exp(i2k_1L) = -1$ (*i.e.* $2k_1L = (2m-1)\pi$, $m = 1, 2, 3\cdots$) and $\exp(-2k_1\beta L) = (1 - w/a)/(1 + w/a)$ (*i.e.* $1 - 2k_1\beta L \simeq 1 - 2w/a$ when $w/a \ll 1$). Hence, we have

$$f = (2m-1)c_1/4L, \tag{S14}$$

$$\beta = \frac{2}{\pi}\frac{w}{(2m-1)a}, \tag{S15}$$

where $m = 1, 2, 3\cdots$ We note that Eqs. (S14) and (S15) are Eqs. (2) and (3), respectively.

## IV. Derivation of Eq. (4)

Assume $k_1 = k_m + \Delta_k/2$, $k_m = (2m-1)\pi/2L$, and $\Delta_k/2 \ll k_m$. When Eq. (S15) is satisfied, Eq. (S11) becomes as $R = [2 + 2\cos(2k_1L)] / [v^2/u^2 + u^2/v^2 + 2\cos(2k_1L)]$, where $u = 1 - w/a$ and $v = 1 + w/a$. Thus, the condition for $R = 1/2$ is

$$\cos(2kL) = \left(v^2/u^2 + u^2/v^2\right)/2 - 2 \tag{S16}$$

By using $\left(v^2/u^2 + u^2/v^2\right)/2 - 2 \simeq -1 + 8(w/a)^2$ and $\cos(2k_1L) \simeq -1 + \frac{1}{2}\left(\Delta_k L\right)^2$, Eq. (S16) becomes as $\Delta_k = w/aL$, so that we have $\Delta_k/k_m = 8w/\left[\pi(2m-1)a\right]$ or

$$\frac{\Delta f}{f_m} = \frac{8w}{\pi(2m-1)a}. \tag{S17}$$

We note that Eq. (S17) is Eq. (4).

## V. Details of Simulations

The metasurface shown in the right panel of Fig. 1(a) can be dealt with a coupled mode theory. Using this method, the results in Figs. 1(b)-1(h) can be efficiently obtained.

Simulations of 3D structures (Figs. 2 and 3) and mode profiles of 2D structures (Fig. 1(c)) were implemented using a finite-element method (COMSOL Multiphysics v4.3). Here, the mass density and sound velocity of air were set as 1.29 kg/m$^3$ and 340 m/s, respectively;

the mass density, Young's modulus and Poisson's ratio of polylactic acid (PLA) were set as $1.24 \times 10^3$ kg/m$^3$, 3.5 GPa and 0.4, respectively. Since PLA and air are very different in density, simulated resonant frequencies change slightly ($< 1\%$) when PLA are replaced by rigid body. In experiments, the measured absorption spectra do not change when PLA are replaced by Acrylonitrile butadiene styrene (ABS).

In the frequency ranges studied in Figs. 3(d) and 3(e), the fundamental ($m = 1$) resonance dominates, so that Eqs. (7) and (8) can reduce as

$$A = \frac{4Q_a^{-1}Q_r^{-1}}{4(f/f_1 - 1)^2 + (Q_a^{-1} + Q_r^{-1})^2}. \tag{S18}$$

By fitting the curves in Figs. 3(d) and 3(e) with this simplified equation, the resonant frequency $f_1$, absorptive quality factor $Q_a$ and radiative quality factor $Q_r$ can be obtained for the $m = 1$ resonance.

## VI. Sample Fabrications

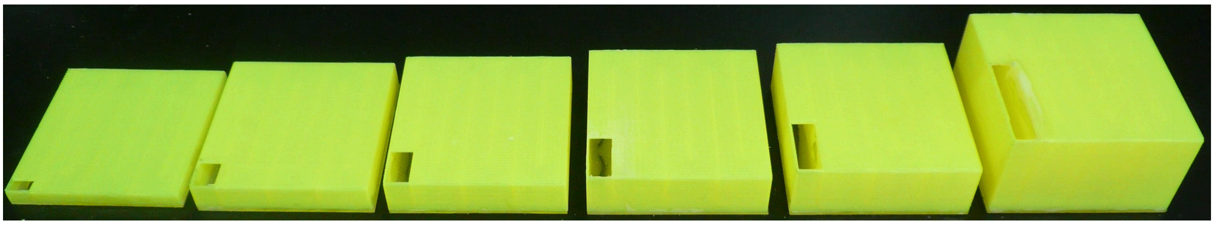

The sample shown in the left panel of Fig. 2(b) is composed of a bottom part, as shown in the right panel of Fig. 2(b), and a square cover. The two parts were first fabricated with PLA by 3D printing technology, and then agglutinated together. Similarly, the sample shown in Fig. 3(a) was also fabricated.

## VII. Characterizations

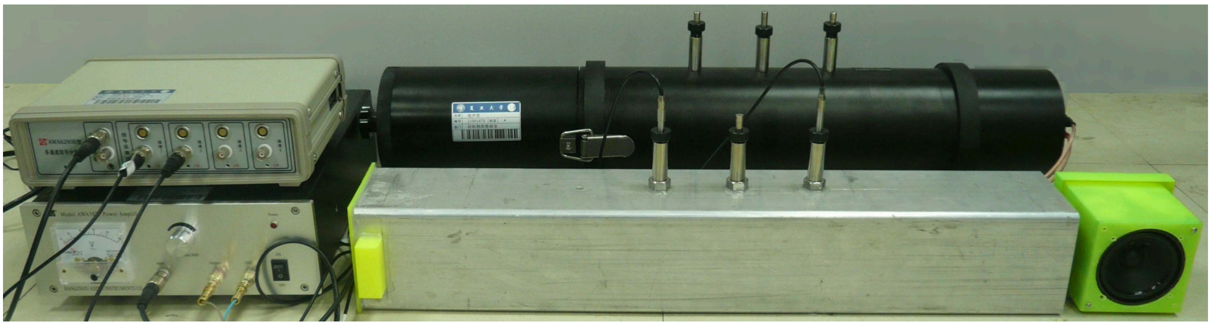

A commercial impedance tube (Hangzhou Aihua, AWA6290T), which complies with ASTM C384-04(2011) and ASTM E1050-12, was applied to measure the absorption of acoustic metasurfaces. Here, the impedance tube has a square cross section with size of 9.05 cm, one (left) closed end and another (right) open end. Two 1/4-inch condensed microphones were situated at designated positions to sense local pressure. For each measurement, a unit cell of the metasurface was first placed at the left end of the tube, and a cubic box with loudspeaker was then placed at the right end (so that the right end is also closed). The loudspeaker was fed with a sinusoidal signal of which the frequency increases with increasing time. By analyzing the signals from microphones, the absorption of the unit cell can be obtained by $A = 1 - |r|^2$, where $r$ is the reflection coefficient of the unit cell.
